# Supplementary material for: Isotropic-nematic transition of self-propelled rods in three dimensions
Source: arXiv:1801.08790 ancillary file (2018-06-28)
Supplement: Supplementary file 1 [file supplementary_material.pdf]

# Isotropic-nematic transition of self-propelled rods in three dimensions: Supplementary information

M.C. Bott,<sup>1</sup> F. Winterhalter,<sup>2</sup> M. Marechal,<sup>2</sup> A. Sharma,<sup>3</sup> J.M. Brader,<sup>1</sup> and R. Wittmann<sup>1</sup>

<sup>1</sup>*Soft Matter Theory, University of Fribourg, CH-1700 Fribourg, Switzerland*

<sup>2</sup>*Institut für Theoretische Physik, Universität Erlangen Nürnberg, 91058 Erlangen, Germany*

<sup>3</sup>*Leibniz-Institut für Polymerforschung Dresden, 01069 Dresden, Germany*

In this supplementary information we present additional simulation data for the three-dimensional Gay-Berne system, a short discussion of related results we obtained for a two dimensional Gay-Berne system and provide finite size analysis for the hard spherocylinder system. In the following, we provide an outline of this document and a brief summary of the main conclusions that can be drawn from each section.

In Sec. I we show an extended phase diagram including the complete parameter space we covered in our computations. Moreover, we denote each state point for which we performed a simulation run and discuss some subtleties. In Sec. II we present results for the three dimensional Gay-Berne model in a larger system. This serves to support the statements in the main text that the polar state is a finite-size effect, whereas the nematic phase boundary remains invariant. Moreover, the fluctuations over simulation time of the order parameters are shown to decrease. In Sec. III we compare the time series of the order parameter for the (smaller) three dimensional system at different activities. This serves to corroborate the argumentation in the main text that despite, or rather because of, significant fluctuations in the active nematic phase, the IN phase boundary can be determined in a relatively small system. In Sec. IV we calculate the variance of the order parameter to show that the resulting error bars do not exceed the symbol size in the plots of the main paper. In Sec. V the two dimensional Gay-Berne results are presented. This serves to emphasize that the effects observed in three dimensions of activity on the IN transition would be observable (if there exists an active nematic phase at all) only in a very small range of (small) activities. Finally in Sec. VI we provide a finite size analysis for the hard spherocylinder model by presenting the order parameter for different system sizes.

## I. DETAILED PHASE DIAGRAM

As presented in the main text, we carried out simulations of rod-like repulsive Gay-Berne particles at fixed temperature  $k_B T / \epsilon_0 = 0.65$  with aspect ratio  $\kappa = \sigma_s / \sigma_e = 1/3$  and  $\kappa' = \epsilon_e / \epsilon_s = 5$ . The interaction exponents  $\mu$  and  $\nu$  are chosen as  $\mu = 2$  and  $\nu = 1$ . Since the particles are soft, there is no clear-cut definition of a packing fraction  $\eta$ . For our presentation, we define  $\eta = N V_E / V$ , with  $V$  being the volume of the simulation box and  $V_E = 4\pi\sigma_0^3 / (3\kappa)$  the volume of one ellipsoidal particle with long axis  $\kappa^{-1}\sigma_0$ .

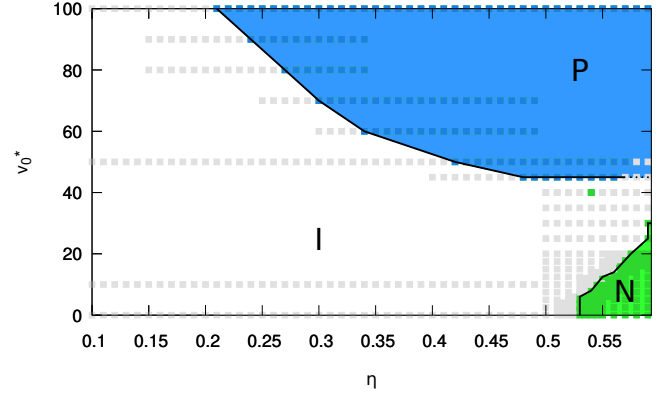

FIG. 1. Phase diagram for a wide range of activities and densities. Each point in the parameter space for which we performed simulations is marked with square. Values above the nematic threshold value  $S_t = 0.35$  are marked green and values above the polar threshold value  $P_t = 0.55$  are marked blue.

In Fig. 1 we show the phase diagram for a wide range of activities and densities. In addition to the phase boundaries we show each parameter for which we performed simulations to determine the transition. Average values above the nematic threshold value  $S_t = 0.35$  are marked in green and values above the polar threshold value  $P_t = 0.55$  are marked in blue. On this basis we are able to separate the density-activity parameter space into the different areas. Most extensively we studied parameters around the IN phase boundary to resolve the latter precisely. The polar area does not represent a true equilibrium phase and is not the main interest of our study, which is why we chose to perform fewer simulation measurements at the activities and densities in question. Around the transition area between the isotropic and the polar area we experience high fluctuations, especially at high densities. This makes it difficult to precisely assign those parameters to polar states or the isotropic phase, which is why we experienced a few exceptions in polar area of Fig. 1. However, this region of the phase diagram is dominated by finite-size effects, which we demonstrate in the following.

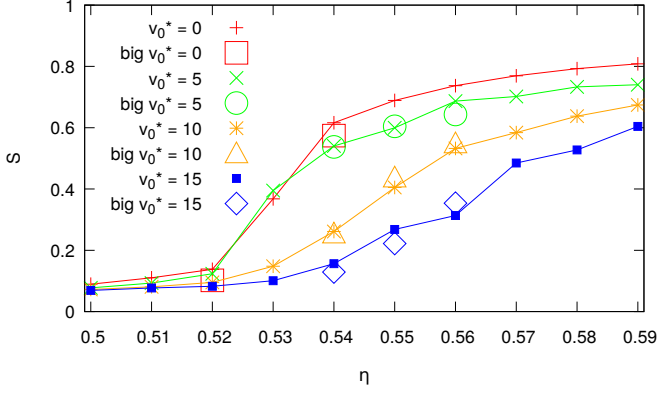

FIG. 2. Average nematic order parameter in three dimensions for a passive ( $v_0^* = 0$ ) and an active system ( $v_0^* = 5, 10, 15$ ) as a function of the packing fraction for two different system sizes  $N = 500$  and  $N = 1000$ . The average order parameter for both system sizes are in fair agreement, which indicates the independence of the IN phase boundary from the system size.

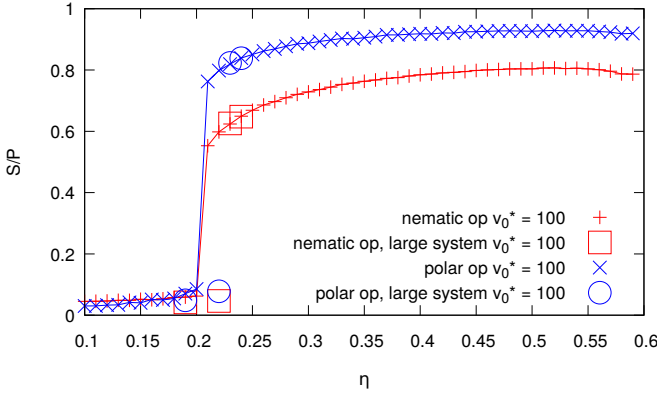

FIG. 3. Average nematic and polar order parameter in three dimensions for an active system ( $v_0^* = 100$ ) as a function of the packing fraction for two different system sizes  $N = 500$  and  $N = 1000$ . The average polar and nematic order parameter show a jump at higher packing fraction for the larger system size.

## II. LARGER SYSTEM SIZE IN THREE DIMENSIONS

In addition to the simulations of the Gay-Berne model with  $N = 500$  particles presented in the main text we performed simulations of larger systems with  $N = 1000$  particles to check whether the IN phase boundary is influenced by system size. In Fig. 2 we show the average order parameter as a function of the packing fraction for both a system of  $N = 500$  and  $N = 1000$  particles for activities  $v_0^* = 0, 5, 10$  and  $15$ . The measurements performed for the larger system indicate that the IN phase boundary is independent of the system size, as the aver-

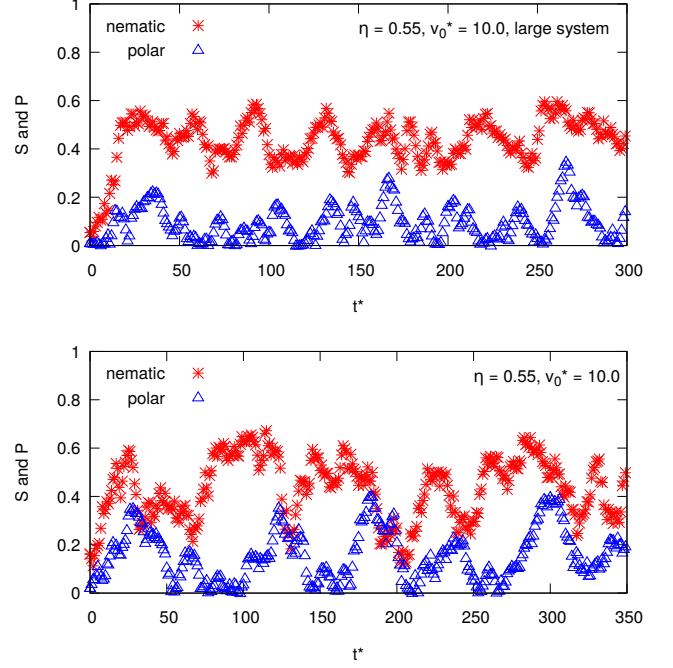

FIG. 4. Time series of nematic  $S$  and polar  $P$  order parameter in three dimensions at packing fraction  $\eta = 0.55$  and activity  $v_0^* = 10$  for a system with  $N = 1000$  and  $N = 500$  particles. We observe that for larger system sizes fluctuations decrease.

age nematic order parameters for both system sizes are in fair agreement. The polar state, however, is clearly influenced by system size, as we see in Fig. 3. The onset of the jump of both the polar and the nematic order parameter is shifted to higher densities for a given activity. This consistently verifies that the polar state in our finite-size simulation does not represent a true equilibrium phase.

In Fig. 4 we show the nematic and polar order parameter as a function of simulation time for a state point at packing fraction  $\eta = 0.55$  and activity  $v_0^* = 10$ , close to the IN phase boundary but still in the nematic phase. Comparing the large system with  $N = 1000$  particles to the smaller one with  $N = 500$  particles, we notice that the fluctuations around the average values, which are in agreement for both system sizes, decrease for the larger system. Of course, an even larger system would be required to properly characterize the active nematic phase. However, even for the chosen system sizes, the IN transition can be properly identified, as we discuss in the following.

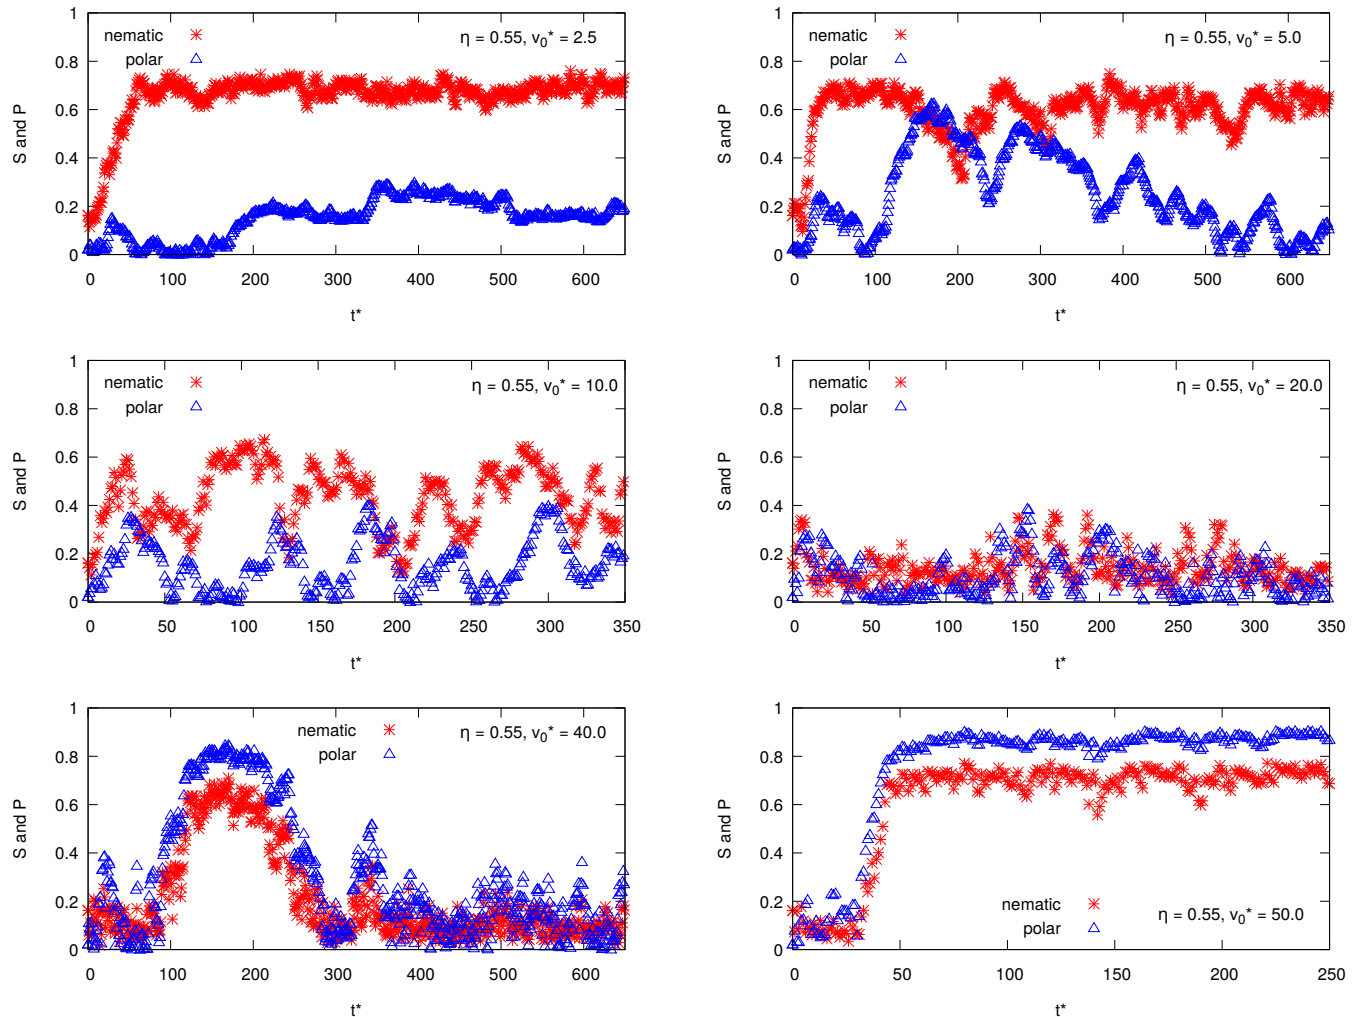

FIG. 5. Time series of nematic  $S$  and polar  $P$  order parameter (3D system) at packing fraction  $\eta = 0.55$  of our numerical simulations, initialized in an isotropic state, for various values of the activity  $v_0^*$ .

### III. TIME SERIES OF THE ORDER PARAMETER IN THREE DIMENSIONS

In Fig. 5 we show the numerical measurements of the nematic  $S$  and polar  $P$  order parameter as a function of simulation time for various activities. We chose a packing fraction  $\eta = 0.55$  corresponding to a passive nematic state. All time series of nematic and polar order parameter have very small initial values. This is due to the fact that we have used isotropic initial conditions and only once the system reached an equilibrium state we started computing the average order parameter. In addition to the isotropic initial conditions we also used polar initial conditions (not shown) for some state points which are in the nematic phase. Since both initial conditions lead to nematic configurations, the average order parameters are independent of the initial conditions.

For low activities ( $v_0^* = 2.5$ ) we observe in Fig. 5 only

insignificant fluctuations in the two order parameters and the active nematic phase can be properly described. Initially, the fluctuations increase markedly as we go to higher activities. At  $v_0^* = 5$  the fluctuations are mainly in the polar order parameter, so that the time-average of  $S$  is well-defined. The anti-correlation between the instantaneous values of  $S$  and  $P$  at  $v_0^* = 10$  indicates finite-size effects, as we have already established in Fig. 4. Therefore, at this activity, we still describe the system as nematic, although the order parameter is strongly fluctuating. After the predicted IN phase boundary is crossed the fluctuations decrease significantly. This observation is a strong indicator for the presence of a phase transition (if we assumed that there was only a single state, one would expect that the fluctuations increase throughout the sweep of the activity). The state point with  $v_0^* = 20$  is thus clearly isotropic.

It is well known that there are no finite-size effects in

the isotropic phase until a critical (activity-dependent) system size, which allows a polar cluster to span the whole volume. For our simulation box, this is represented by the observed boundary of the polar state. Only as we approach this boundary at ( $v_0^* = 40$ ) fluctuations (around small values of  $S$  and  $P$ ) increase again, but now both order parameters fluctuate uniformly, which clearly differs from the behavior associated with the active nematic phase. Once the system reaches the polar state ( $v_0^* = 50$ ) the fluctuations are mainly gone, because the whole system is spanned by a polar cluster.

#### IV. STANDARD DEVIATION OF THE NEMATIC ORDER PARAMETER

To provide a simple check for the error of the nematic order parameter at finite activity, we chose the activities  $v_0^* = 5$  and  $v_0^* = 10$  and calculated the variance for the packing fraction  $\eta = 0.52, 0.55$  and  $0.58$  in the repulsive Gay-Berne model. This represents states in the isotropic phase, in the transition region and in the nematic phase, respectively. For each parameter we performed  $n = 5$  independent simulation runs over  $t^* = 400$  Brownian seconds for  $v_0^* = 10$  and  $t^* = 350$  Brownian seconds for  $v_0^* = 5$  and calculated the standard deviation  $\sigma$  as

$$\sigma = \sqrt{\frac{\sum_{i=1}^n (S_i - S_{\text{avg}})^2}{n-1}}, \quad (1)$$

where  $S_i$  denotes the order parameter determined of each measurement and  $S_{\text{avg}}$  the average order parameter of the five measurements. In figure 6 we show again the nematic order parameter for the passive system and at activities  $v_0^* = 5, 10$ . Here, the variance of the order parameter is included in form of an error bar. In particular in the isotropic and in the nematic phase the error bars are very small, in fact smaller then the regular symbol size of the plot.

Our results indicate that for very small activities ( $v_0^* \leq 0.1$ ) one can still observe nematic ordering. This means that, as in the passive case, depicted in Figs. 7a and 7b, we see a clearly isotropic phase at low densities in Fig. 7c and nematic alignment at higher densities in Fig. 7d, re-

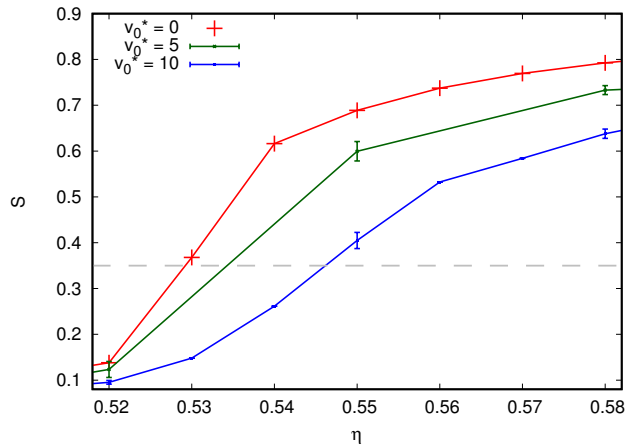

FIG. 6. Nematic order parameter  $S$  as a function of packing fraction  $\eta$  for the passive system and active systems at  $v_0^* = 5$  and  $v_0^* = 10$ . For the active system we included the variance of the nematic order parameter in form of error bars for three different state points. In the isotropic phase ( $\eta = 0.52$ ) and the nematic phase ( $\eta = 0.58$ ) the error bars are much smaller then the regular symbol size used in the rest of the paper. Even in the transition region between the two phases ( $\eta = 0.55$ ) the error bar remains comparable to the symbol size.

#### V. TWO-DIMENSIONAL SYSTEM

In two dimensions we performed simulations of the WCA-Gay-Berne model with  $N = 2000$  particles at fixed temperature  $k_B T / \epsilon_0 = 1$ . We chose an aspect ratio  $\sigma_e / \sigma_s = \kappa = 5$  and the ratio of the interaction strength as  $\epsilon_e / \epsilon_s = \kappa' = 1/5$ . The interaction exponents were chosen as  $\mu = 1$  and  $\nu = 2$ . In the two dimensional case the packing fraction is given as  $\eta = \pi \sigma_e \sigma_s \rho / 4$ . Generally, the two dimensional system takes much longer to equilibrate than in three dimensions, therefore longer simulation runs are needed to create equivalent statistics. Since there is already a significant amount of work on SPR in two dimensions, we only discuss the different simulation snapshots in Fig. 7 and the time-averaged order parameters as a function of the packing fraction in Fig. 8 with the aim to qualitatively argue about the influence of a small amount of activity on nematic order. We do not seek to draw a full phase diagram, conclude on finite-size effects at higher activity or argue about the stability of the nematic phase in general, so that the relatively low amount of statistics presented here is sufficient.

spectively. In this activity regime, we observe in Fig. 8a that the nematic order parameter is always quite close to its values for the passive system and the polar order parameter stays overall very low. If we further increase the activity the system becomes more and more inhomogeneous.

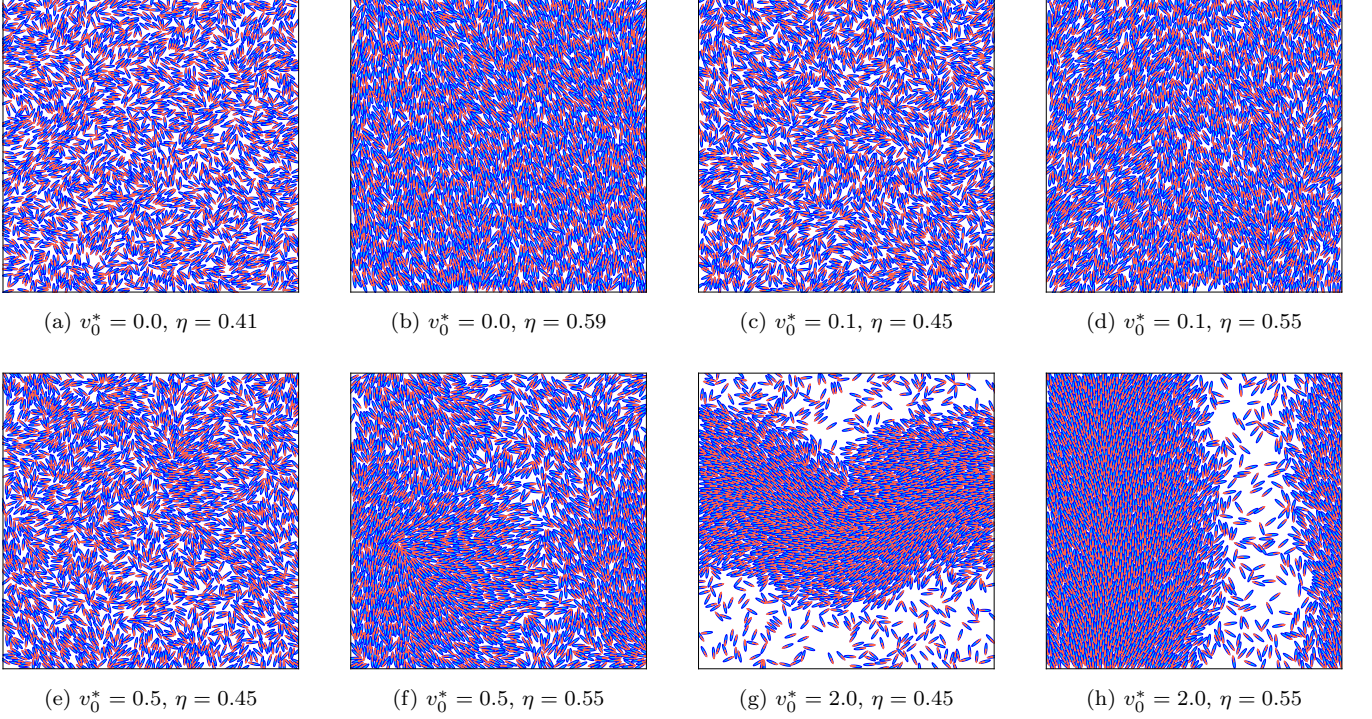

FIG. 7. Simulation snapshots of two dimensional Gay-Berne system for various activities and densities. Snapshot (7a) shows an isotropic state at  $\eta = 0.41$  and the snapshot (7b) a nematic state at  $\eta = 0.59$  both for the passive system. With a very small amount of activity  $v_0^* = 0.1$  the snapshots still indicate isotropic (7c) ordering at  $\eta = 0.45$  and nematic ordering (7d) at  $\eta = 0.55$ . At activity  $v_0^* = 0.5$  we observe weak (at  $\eta = 0.45$  (7e)) and strong (at  $\eta = 0.55$  (7f)) number fluctuations along with local polar clusters. For even higher activities  $v_0^* = 2.0$  both packing fractions  $\eta = 0.45$  and  $\eta = 0.55$  result in a band-like structure in snapshots (7g) and (7h).

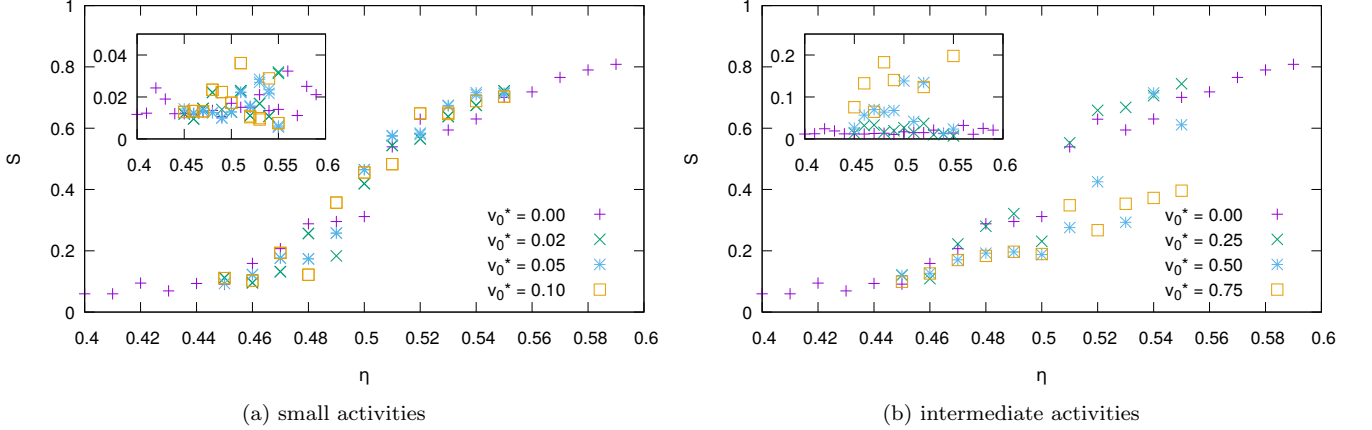

FIG. 8. Nematic and polar (inset) order parameter as a function of packing fraction for various activities in two dimensions. As a reference each plot contains the order parameters of the passive system. We display the behavior for (8a) small activities,  $v_0^* \in \{0.02, 0.05, 0.1\}$ , where the behavior is similar as for the passive system and (8b) intermediate activities,  $v_0^* \in \{0.25, 0.5, 0.75\}$ .

geneous, which already becomes apparent for  $v_0^* = 0.5$  in Figs. 7e and 7f and results in the polar bands at  $v_0^* = 2$  depicted in Figs. 7g and 7h, dominated by finite-size effects. These number fluctuations invalidate the characterization of the active system by means of global order

parameters, as shown in Fig. 8, for high activities  $v_0^* > 1$ .

In conclusion, when comparing these findings to the three-dimensional results of the main text, we observe that in two dimensions the activity destroys nematic order much more rapidly, i.e., at much smaller values of  $v_0^*$ .

Already for activities above  $v_0^* > 0.5$  an active nematic phase, as described in the main text, can definitively no longer be observed in two dimensions. We are not aware of any previous simulation study resolving this parameter range and thus arguing about the possibility to find an active nematic phase in two dimension. Another important difference related to the dimensionality, are the

strong fluctuations in the local density, which are absent in three dimensions, where the system appears to be homogeneous even at much higher activities. Therefore, our preliminary 2D results reported here do not provide a conclusive answer on whether such a 2D nematic phase at low activity is truly stable under fluctuations with a wave-length larger than our system size.

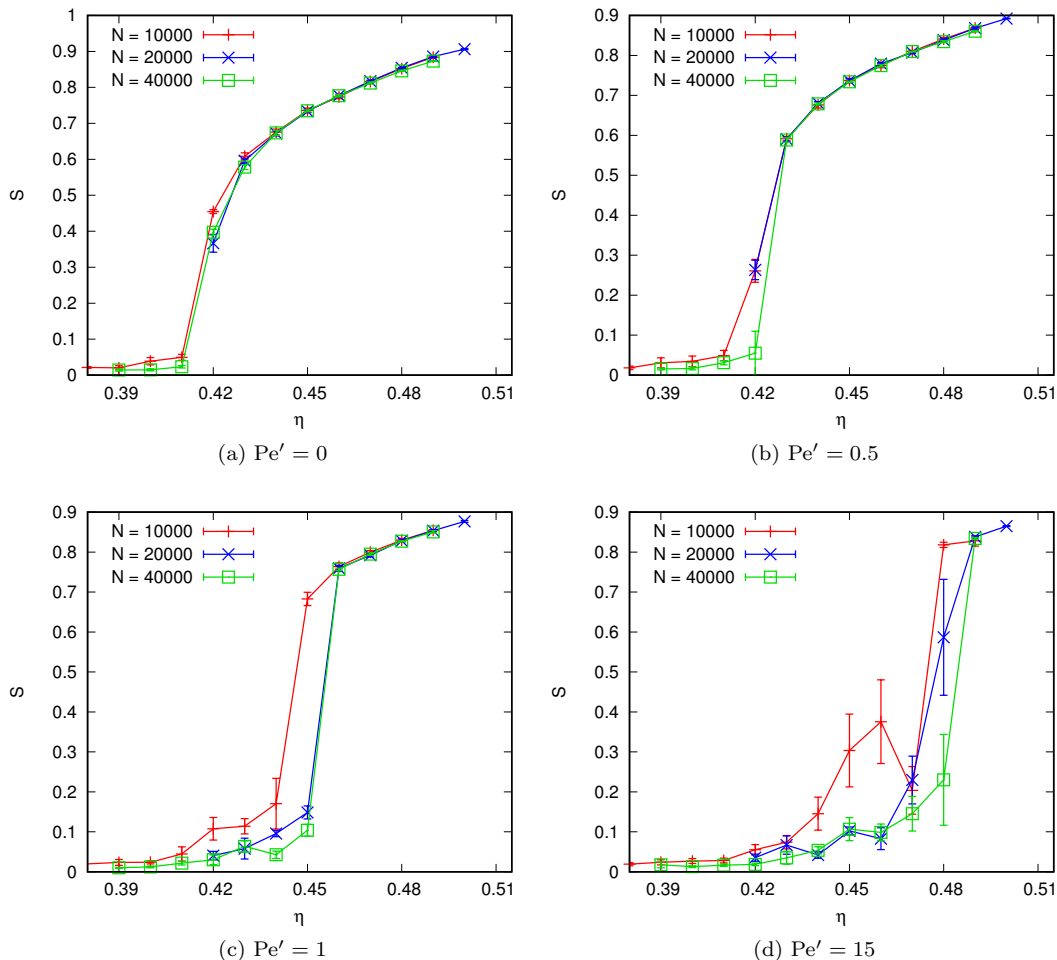

FIG. 9. The nematic order parameter versus the packing fraction for three system sizes,  $N = 10\,000$ ,  $N = 20\,000$  and  $N = 40\,000$  and propulsion speeds given by the following Peclet numbers  $Pe'$ :  $Pe' = 0$  (a),  $Pe' = 0.5$  (b),  $Pe' = 1$  (c) and  $Pe' = 1.5$  (d).

## VI. FINITE SIZE ANALYSIS FOR THE SPHEROCYLINDER MODEL

For the HSC model we performed simulations for  $N = 10\,000$ ,  $N = 20\,000$  and  $N = 40\,000$  particles. The nematic order parameters for these three system sizes are compared to each other in Fig. 9. We see little finite size effects, except that (obviously) the nematic order and the corresponding error bars decrease with increasing system size in the isotropic phase (since the nonzero value is purely a standard finite size effect due to the presence

of finite nematic or polar clusters). The error bars are a measure of the standard deviation. Each error bar was obtained by dividing the data of a single simulation into five blocks and using the five averages of those blocks in standard error analysis (see also the supplementary file about the repulsive Gay-Berne model), assuming the five data points thus obtained are independent. The large ‘hump’ in Fig. 9d for  $Pe' = 1.5$  in the smallest system is probably due to a large polar cluster; it depends critically on both the shape and the size of the simulation box.
